# Supplementary material for: GSGS: A Computational Framework to Reconstruct Signaling Pathways from Gene Sets
Source: arXiv:1101.3983 source file (2011-10-13)
Supplement: Supplementary file 1 [file supplementary.pdf]

# Supplementary Material

## 1 Burn-in state

To determine an appropriate burn-in state, we translated the procedure described in [Gelman *et al*, 2003] [Givens *et al*, 2005] for the standard Gibbs sampling approach, in our framework. We compared the within-chain and between-chain variances for three quantities of our interest sensitivity, specificity and PPV using this procedure. Let us fix the burn-in state as  $B$  and the number of networks (pathways) sampled after burn-in as  $N$ , in a total of  $J$  ( $\geq 2$ ) independent runs of Gene Set Gibbs Sampler. For the parameter of interest  $X$ , define

$$\bar{x}_j = \frac{1}{N} \sum_{t=B+1}^{B+N} x_j^{(t)}$$

where  $x_j^{(t)}$  is the parameter value at the  $t^{th}$  iteration of the  $j^{th}$  chain  $j = 1, \dots, J$ , and

$$\bar{x} = \frac{1}{J} \sum_{j=1}^J \bar{x}_j.$$

Within-chain variance for the  $j^{th}$  chain and between-chain variance are given by

$$s_j^2 = \frac{1}{N-1} \sum_{t=B+1}^{B+N} (x_j^{(t)} - \bar{x}_j)^2$$

and

$$B_v = \frac{N}{J-1} \sum_{j=1}^J (\bar{x}_j - \bar{x})^2$$

respectively. Let us write  $W_v$  as the average of estimated within-chain variances, i.e.

$$W_v = \frac{1}{J} \sum_{j=1}^J s_j^2$$

and define

$$R = \frac{\frac{N-1}{N} W_v + \frac{1}{N} B_v}{W_v}.$$

If all the chains are stationary then the numerator and denominator in  $R$  estimate the variance of  $X$ . It is clear that as  $N \rightarrow \infty$ ,  $\sqrt{R} \rightarrow 1$ . In practice if  $\sqrt{R} < 1.2$ , the choice of  $B$  and  $N$  is acceptable. Otherwise, either  $B$  or  $N$  or both should be increased.

## 2 Set-up for Data Analysis

**GSGS:** For the *E. coli* and *In Silico* networks

- All IFGS's were generated using Algorithm 2.
- There were a total of 125 and 57 IFGS's of length  $\geq 3$  for the *E. coli* and *In Silico* networks, respectively.
- There were a total of 62 and 37 directed genes pairs representing the true edges in the *E. coli* and *In Silico network*, respectively. These pairs served as prior knowledge.

- Number of independent runs of Gene Set Gibbs Sampler (Algorithm 1) was set at 100.
- The burn-in state was set at 500.
- A total of 500 networks were sampled after burn-in state. To determine if the burn-in state is appropriate, we computed  $W_v$ ,  $B_v$  and  $R$  for sensitivity, specificity and PPV, by considering every  $k^{th}$  network among 500 signaling pathways, for  $k = 2, \dots, 10$ . The computations were based on 20 independent runs of our GSGS algorithm. With the chosen set of parameters,  $\sqrt{R}$  was found approximately equal to one, for three quantities of interest. However, we did not observe a significant change by summarizing sensitivity, specificity and PPV from all 500 networks. It was also observed that there is no much variation in  $W_v$  calculated using the networks after burn-in state, from different Gene Set Gibbs Sampler runs (see Fig. 2 below).

**K2:** It is the standard K2 approach implemented in BNT. The existing implementations can be modified to incorporate prior knowledge, i.e. to generate a partially known ordering of nodes and select parents of each node based on this ordering.

In case of continuous data

- Expression levels were simulated from Gaussian distribution using BNT.
- Number of simulation runs was set at 100.
- Number of samples in data sets was set at 20, 30, 40 and 50.
- The scoring function was set as BIC.
- Maximum number of parents allowed for a node was set at 3.

In case of discrete data

- Discrete samples were generated from the output of Algorithm 2. Each IFGS was represented by a binary sample based on the absence (1) or presence (2) of a gene in the set.
- Number of simulation runs was set at 100.
- The scoring function was set as Bayesian scoring.
- Maximum number of parents allowed for a node was set at 3.

All other parameters were set as default.

**MCMC:** It is the Metropolis-Hastings (MH) approach implemented in BNT. In the presence of prior knowledge, we do not alter prior known edges to generate neighboring networks.

For continuous data

- Expression levels were simulated from Gaussian distribution using BNT.
- Number of simulation runs was set at 100.
- Number of samples was set at 20, 30, 40 and 50.
- The scoring function was set as BIC.
- The burn-in state was set at 500.
- Number of samples collected after burn-in state was set at 500.

For discrete data

- Discrete samples were generated from the output of Algorithm 2 as discussed above.
- Number of simulation runs was set at 100.
- The scoring function was set as Bayesian scoring.
- The burn-in state was set at 500.
- Number of samples collected after burn-in state was set at 500. In order to summarize a network from MCMC approach, an edge present in at least 50% of the networks sampled after burn-in was declared as true edge. However, we did not observe a significant difference on increasing or decreasing this cut-off.

All other parameters were set as default.

## References

- [Gelman *et al*, 2003] Gelman, A., Carlin, J. B., Stern, H. S. and Rubin, D.B. (2003), Bayesian Data Analysis, *Chapman & Hall*.
- [Givens *et al*, 2005] Givens, G. H. and Hoeting, J. A., Computational Statistics, *Wiley Series in Probability and Statistics*.

## 3 Tables and Figures

|      | 0%    | 20%   | 40%   | 60%   | 80%   | 100%  |
|------|-------|-------|-------|-------|-------|-------|
| 20%  | 0.311 | 0.526 | 0.690 | 0.797 | 0.905 | 1     |
| 40%  | 0.376 | 0.581 | 0.720 | 0.825 | 0.907 | 1     |
| 60%  | 0.448 | 0.596 | 0.737 | 0.818 | 0.918 | 1     |
| 80%  | 0.461 | 0.611 | 0.720 | 0.824 | 0.936 | 1     |
| 100% | 0.431 | 0.597 | 0.725 | 0.807 | 0.917 | 1     |
| 120% | 0.448 | 0.591 | 0.715 | 0.790 | 0.913 | 0.999 |
| 140% | 0.412 | 0.555 | 0.686 | 0.788 | 0.900 | 0.992 |
| 160% | 0.414 | 0.539 | 0.661 | 0.762 | 0.884 | 0.995 |
| 180% | 0.403 | 0.499 | 0.644 | 0.745 | 0.867 | 0.989 |
| 200% | 0.372 | 0.497 | 0.612 | 0.717 | 0.858 | 0.982 |

Table 1: F-scores calculated for the GSGS approach with increasing percentage of gene sets in the input (row) and prior knowledge (column). Network: *In Silico*.

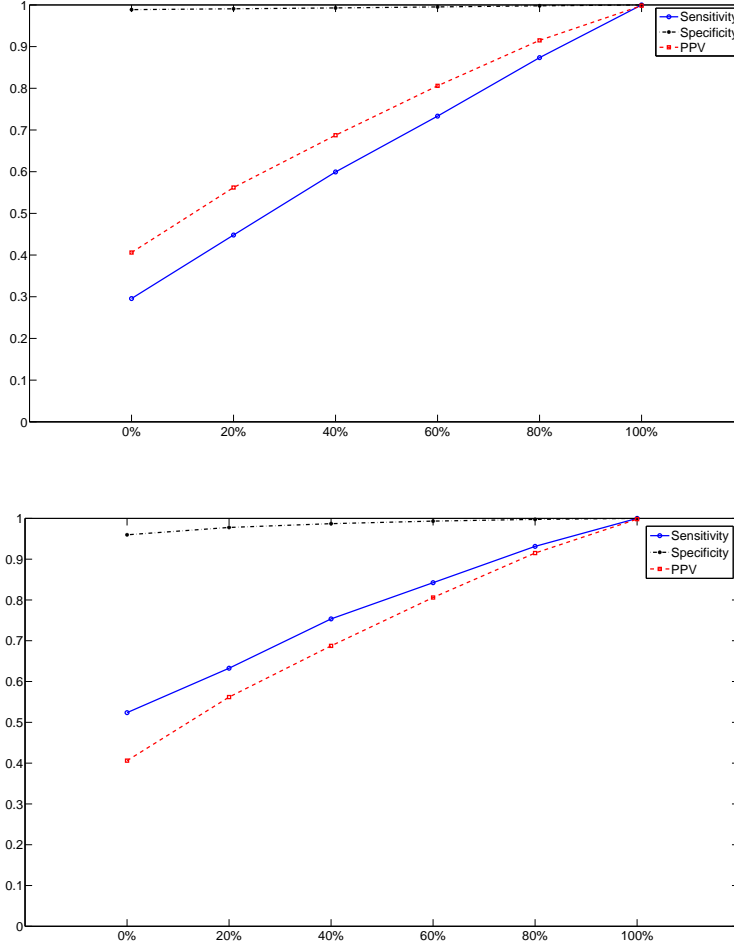

Figure 1: Performance of the proposed GSGS framework with increasing percentage of prior knowledge. Panel 1: *E. coli* network. Panel 2: *In Silico* network. In each panel,  $x$ -axis represents percentage of prior knowledge and  $y$ -axis represents sensitivity, specificity and PPV.

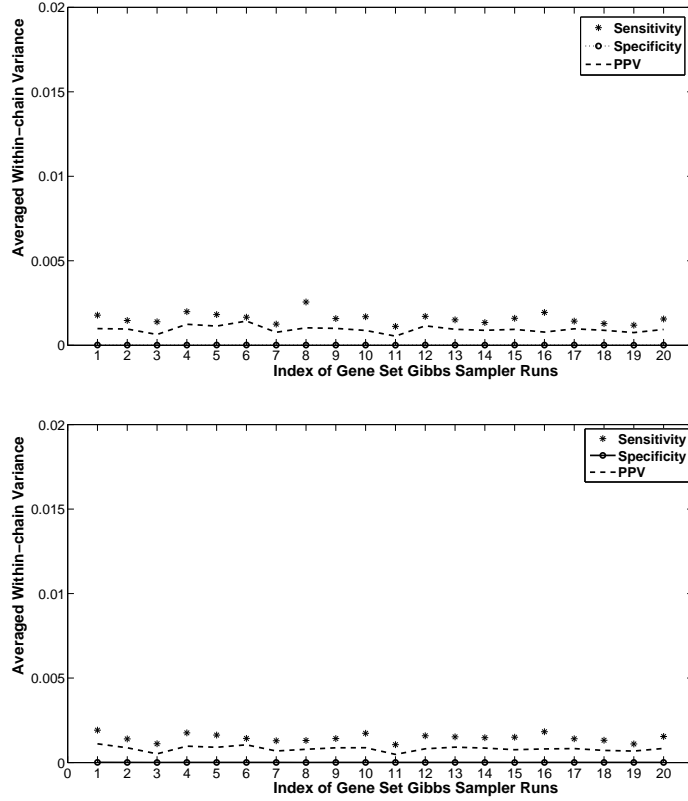

Figure 2: Averaged within-chain variance for sensitivity, specificity and PPV, calculated from 20 independent Gene Set Gibbs sampler runs. Panel 1: *E. coli* Network. Panel 2: *In Silico* Network.

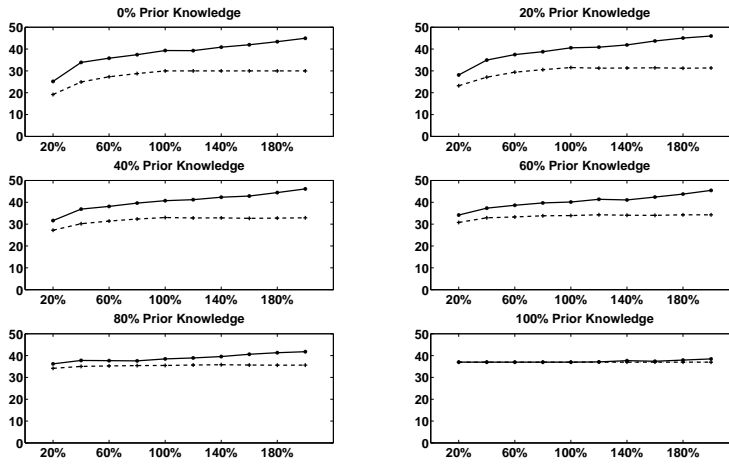

Figure 3: Sensitivity analysis for the GSGS approach with increasing percentage of prior knowledge. Network: *In Silico*. Here,  $x$ -axis represents the percentage of gene sets present in the input and  $y$ -axis plots the total number of edges predicted by GSGS (solid line). The dashed line plots correspond to the ground truth. Here, we have considered only those genes which were present among IFGS's after pruning all gene pairs.

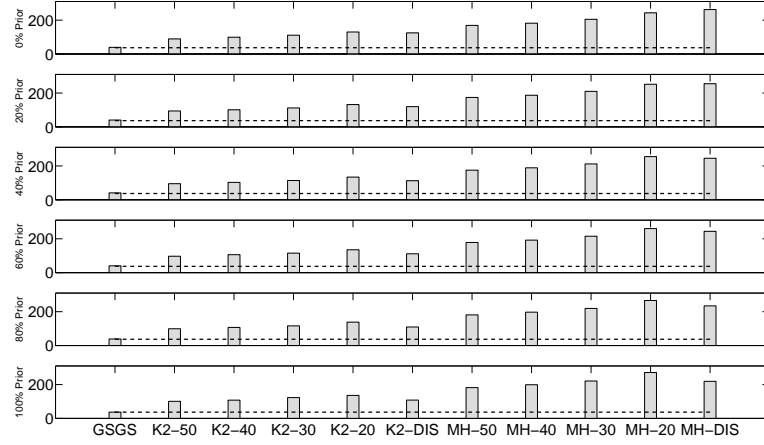

Figure 4: Comparison of the GSGS approach with K2 and MH in terms of total number of predicted edges. Network: *In Silico*. Along  $x$ -axis, “Method-N” represents a Bayesian network method applied to continuous data of sample size N, and “Method-DIS” corresponds to using discrete data.  $y$ -axis represents total number of predicted edges. The dashed line represents ground truth.

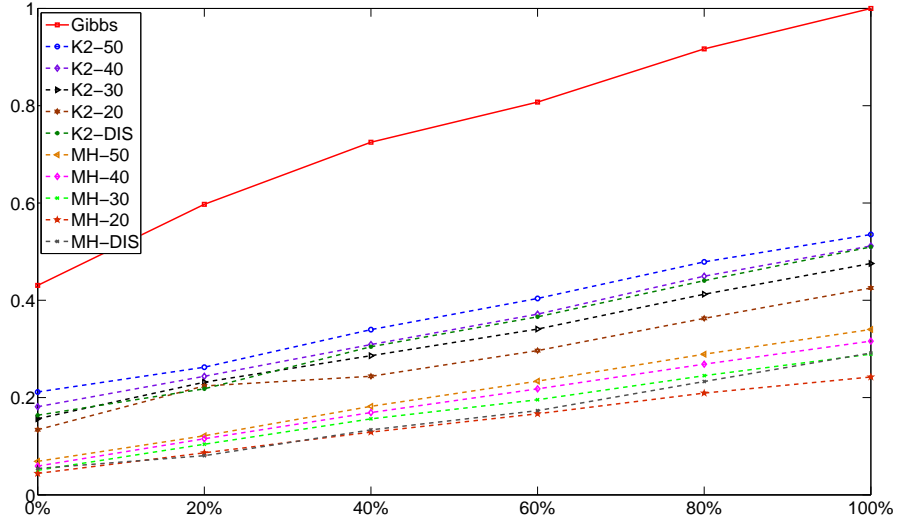

Figure 5: Comparison of the GSGS approach with K2 and MH in terms of F-score. Network: *In Silico*. Here  $x$ -axis denotes the percentage of prior knowledge and  $y$ -axis represents F-scores calculated from different methods. “Method-N” represents a Bayesian network method applied to continuous data of sample size N, and “Method-DIS” corresponds to using discrete data.

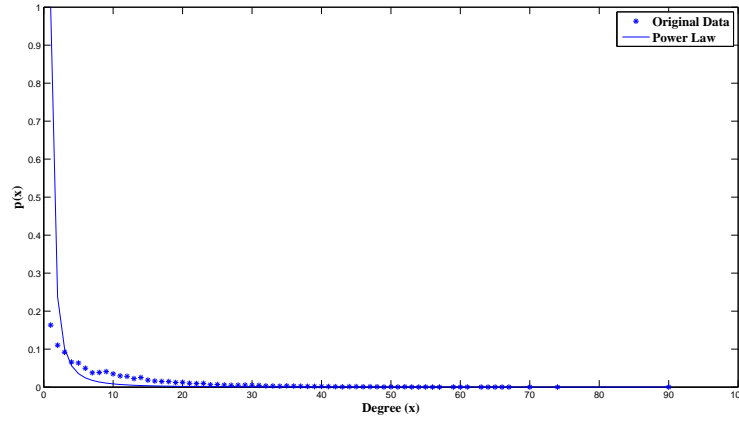

Figure 6: The degree distribution of genes in the C4 gene set compendium approximated by a power-law distribution. Here  $x$ -axis corresponds to a fixed number of gene sets and  $y$ -axis represents the probability of genes belonging to these gene sets

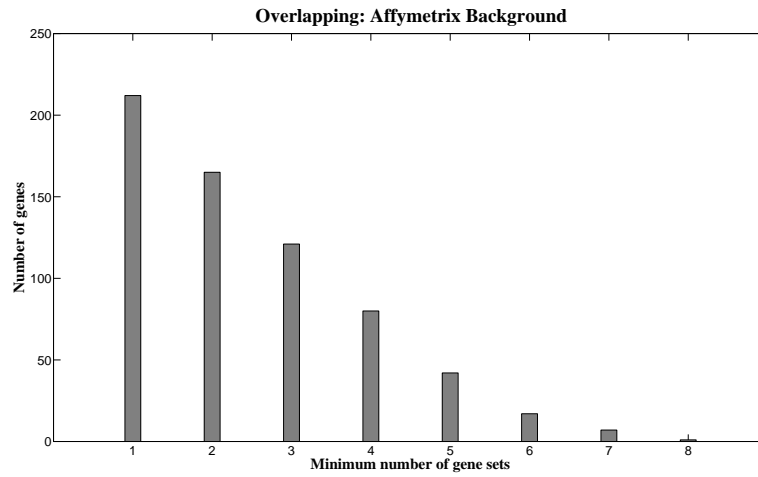

Figure 7: Overlapping among enriched cancer-related gene sets derived using Affymetrix U133 Plus 2.0 background. A bar corresponding to  $(n_1, n_2)$  in the plot means that a total of  $n_1$  genes are shared by at least  $n_2$  gene sets.

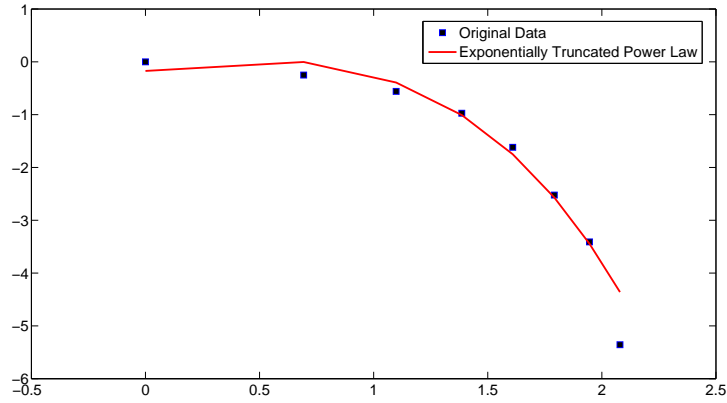

Figure 8: The degree distribution of genes present among cancer related enriched gene sets approximated by an exponentially truncated power law. Here  $x$ -axis corresponds to a fixed number of gene sets and  $y$ -axis stands for the probability of genes belonging to these gene sets, both in log scale.

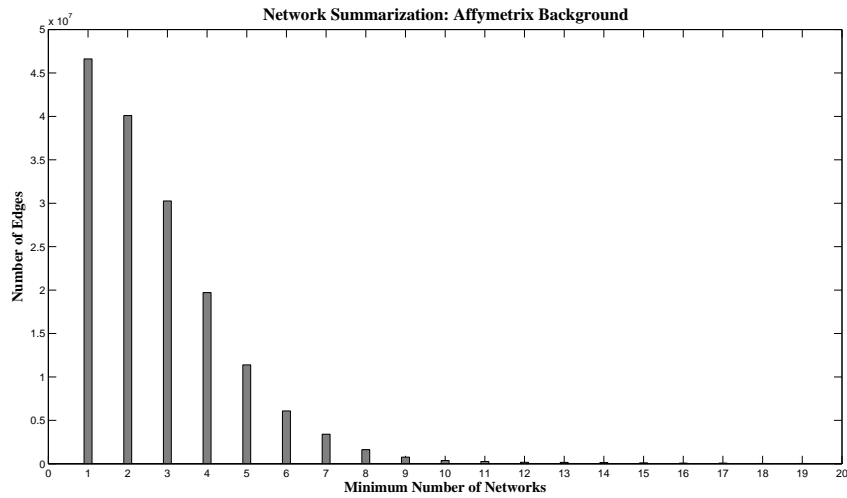

Figure 9: Network Summarization from 20 independent runs of the Gene Set Gibbs Sampler. A bar corresponding to  $(n_1, n_2)$  means that a total of  $n_1$  edges are present in at least  $n_2$  networks.
